# Supplementary material for: DOPE: D-Optimal Pooling Experimental design with application for SARS-CoV-2 screening
Source: arXiv:2103.03706 ancillary file (2021-03-05)
Supplement: Supplementary file 1 [file supplementary_A.pdf]

# Supplementary material A for “DOPE: D-Optimal Pooling Experimental design with application for SARS-CoV-2 screening”

## 1 Algorithms

### 1.1 Gibbs sampler

Our Gibbs sampler is described in Algorithm 1 below.

---

**Algorithm 1** Generate  $L$  “independent” samples from  $\mathbb{P}(\theta|T, \mathbf{d})$  via Gibbs sampling

---

```

1: procedure GIBBS( $\mathbf{d}, T, L, \theta, \tau$ )
2:    $X \leftarrow \text{Zeros}(L, N)$  ▷ Array of zeros of size  $L \times N$ 
3:   for  $n = 1, \dots, L$  do
4:     for  $t = 1, \dots, \tau$  do
5:       for  $i = 1, \dots, N$  do
6:          $p_0 \leftarrow \mathbb{P}(\theta_i = 0, \theta_{-i}|T)\mathbb{P}(\mathbf{d}|\theta_i = 0, \theta_{-i}, T)$ 
7:          $p_1 \leftarrow \mathbb{P}(\theta_i = 1, \theta_{-i}|T)\mathbb{P}(\mathbf{d}|\theta_i = 1, \theta_{-i}, T)$ 
8:          $u \leftarrow U[0, 1]$  ▷ Uniform in  $[0, 1]$ 
9:         if  $\frac{p_0}{p_0+p_1} \leq u$  then
10:            $\theta_i \leftarrow 0$ 
11:         else
12:            $\theta_i \leftarrow 1$ 
13:        $X[n, :] \leftarrow \theta$ 
14:   return  $X$ 

```

---

### 1.2 Hill climbing

Our hill-climbing optimization routine is detailed in Algorithm 2. Perturbations are conducted via the FLIP operator.  $\text{FLIP}(T, i, k)$  flips the membership status of individual  $i$  in pool  $T_k$  in design  $T$ . E.g., if  $T_k = \{1, 4, 9\}$ , then  $\text{FLIP}(T, 1, k)_k = \{4, 9\}$  and  $\text{FLIP}(T, 2, k)_k = \{1, 2, 4, 9\}$ . We consider all perturbations of one and two individuals, as described in Algorithm 2 below. The reason we allow flipping two individuals is to have the possibility of not changing the number of members in a pool. We start the optimization from several

different (random) designs and when optimization ends — choose the design of maximal  $\widehat{\Psi}$ .

---

**Algorithm 2** Returns a design  $T$  maximizing  $\widehat{\Psi}$

---

```

1: function CHOOSERANDOM( $n, k$ )                                ▷ Choose  $k$  elements from  $\{1, \dots, n\}$ 
2: function FLIP( $T, i, k$ )
3:    $T' \leftarrow T$ 
4:   if  $i \in T_k$  then                                         ▷  $T_k$  is the  $k^{\text{th}}$  element of  $T$ 
5:      $T'_k \leftarrow T_k - \{i\}$                                ▷ If  $i$  is in  $T_k$ , remove it
6:   else
7:      $T'_k \leftarrow T_k \cup \{i\}$                              ▷ If  $i$  not in  $T_k$ , add it
8:   return  $T'$ 
9: procedure OPTIMALDESIGN( $K, T', \mathbf{d}'$ )
10:   $T \leftarrow \text{RANDOMDESIGN}(K)$                                ▷ Random start with  $K$  pools
11:   $T_{\text{prev}} \leftarrow \emptyset$ 
12:  while  $T \neq T_{\text{prev}}$  do
13:     $T_{\text{prev}} \leftarrow T$ 
14:    for  $i \in \text{CHOOSERANDOM}(N, 4)$  do
15:      for  $k \in \text{CHOOSERANDOM}(K, 4)$  do
16:         $T_{\text{tmp}} \leftarrow \text{FLIP}(T, i, k)$ 
17:        if  $\widehat{\Psi}(T_{\text{tmp}}; T', \mathbf{d}') > \widehat{\Psi}(T; T', \mathbf{d}')$  then
18:           $T \leftarrow T_{\text{tmp}}$ 
19:        for  $j \in \text{CHOOSERANDOM}(N, 4)$  do
20:           $T_{\text{tmp}} \leftarrow \text{FLIP}(T_{\text{tmp}}, j, k)$ 
21:          if  $\widehat{\Psi}(T_{\text{tmp}}; T', \mathbf{d}') > \widehat{\Psi}(T; T', \mathbf{d}')$  then
22:             $T \leftarrow T_{\text{tmp}}$ 
23:  return  $T$ 

```

---

## 2 Varying $P_{\text{fn}}$ and $P_{\text{fp}}$

We make the comparisons for various  $P_{\text{fn}}$  and  $P_{\text{fp}}$  values in the range  $0.05 \leq P_{\text{fn}} \leq 0.2$  and  $P_{\text{fp}} \in \{0.01, 0.05\}$  in Figure 1 and Figure 2. Population size  $N = 10$ .

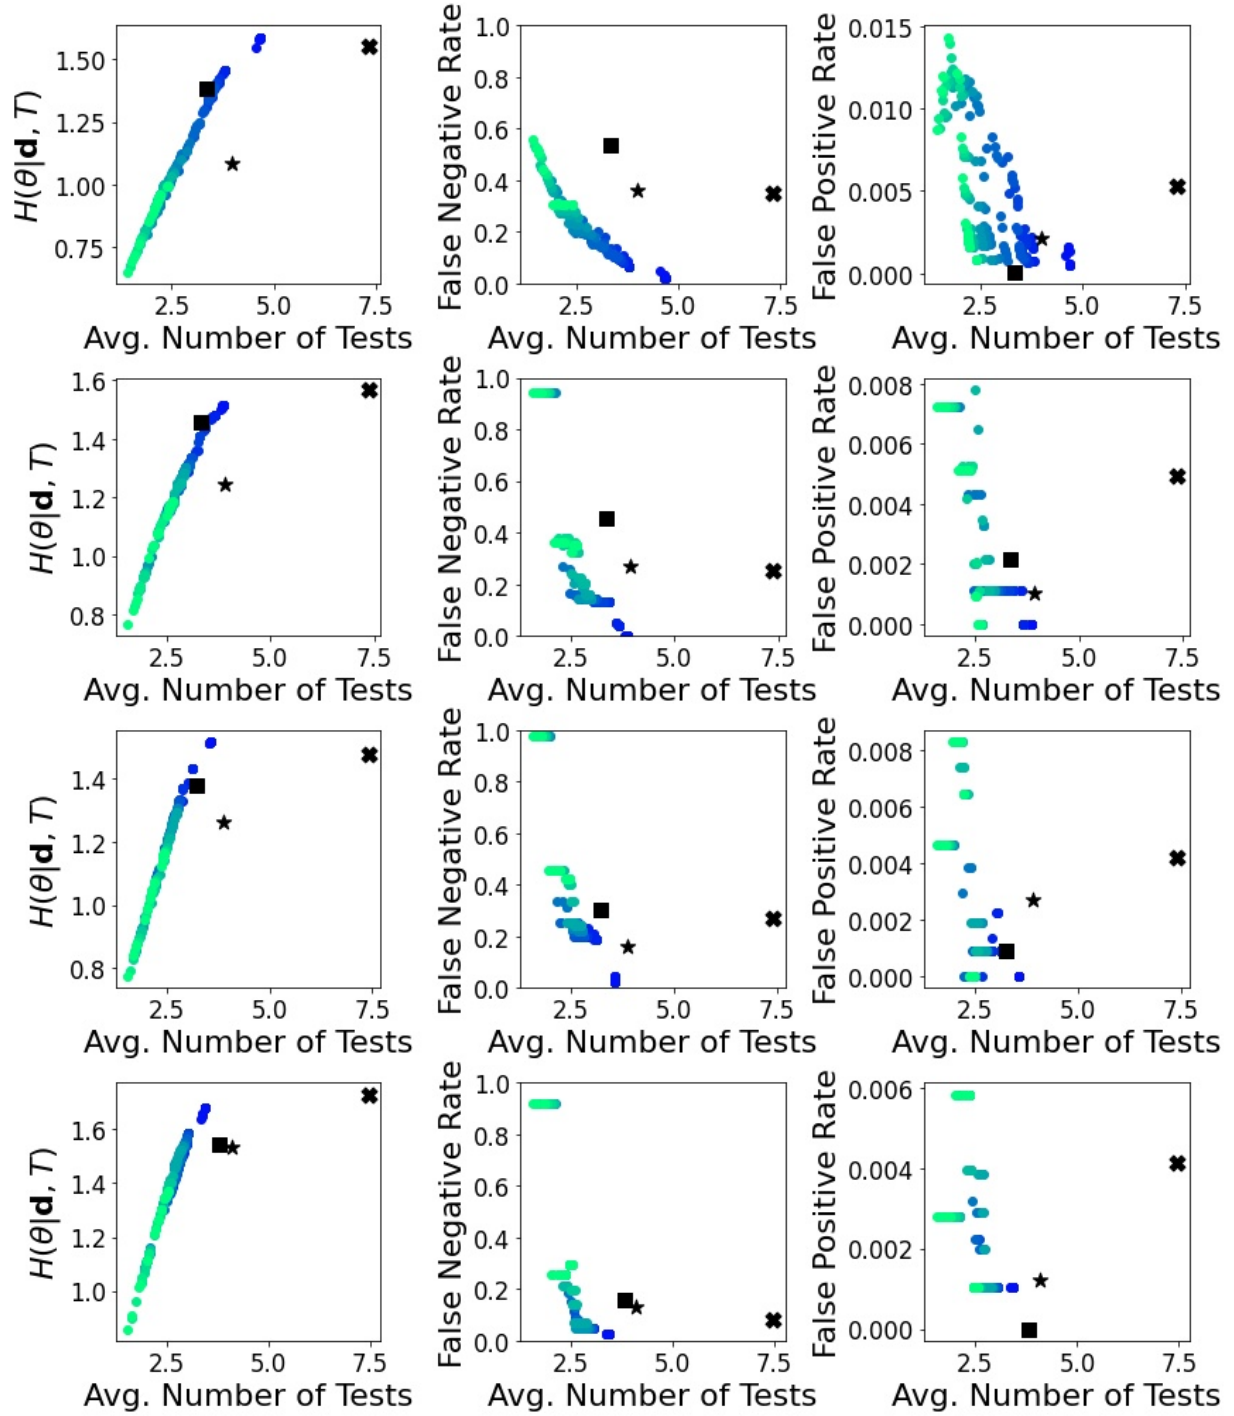

Figure 1: Sensitivity analysis for DOPE. Constant  $P_{fp} = 0.01$  and (top to bottom)  $P_{fn} = 0.2, 0.15, 0.1, 0.05$ . DOPE still dominates its competition.

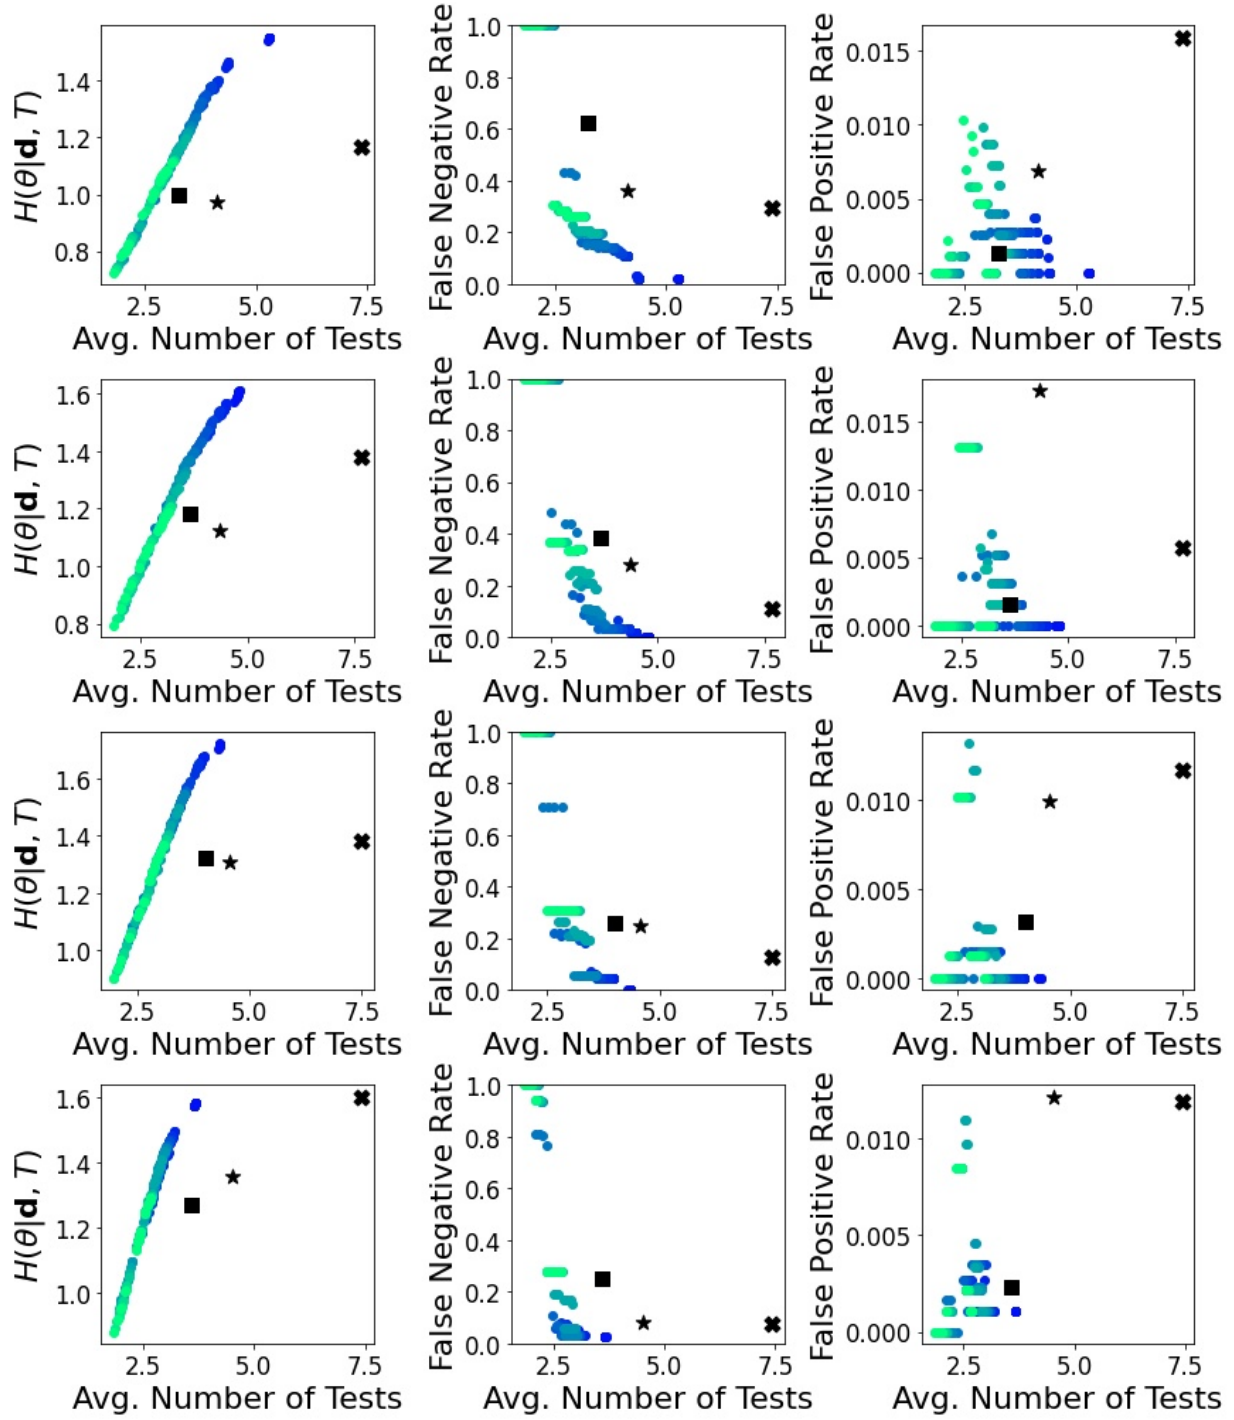

Figure 2: Sensitivity analysis for DOPE. Constant  $P_{fp} = 0.05$  and (top to bottom)  $P_{fn} = 0.2, 0.15, 0.1, 0.05$ . DOPE still dominates its competition.

### 3 Disconnected population

A large testing facility may not have the resources to track connectivity between arriving individuals. Below, we show simulation results for an assumed iid (independent identically distributed) population. DOPE still dominates Dorfman, recursive and matrix pooling.

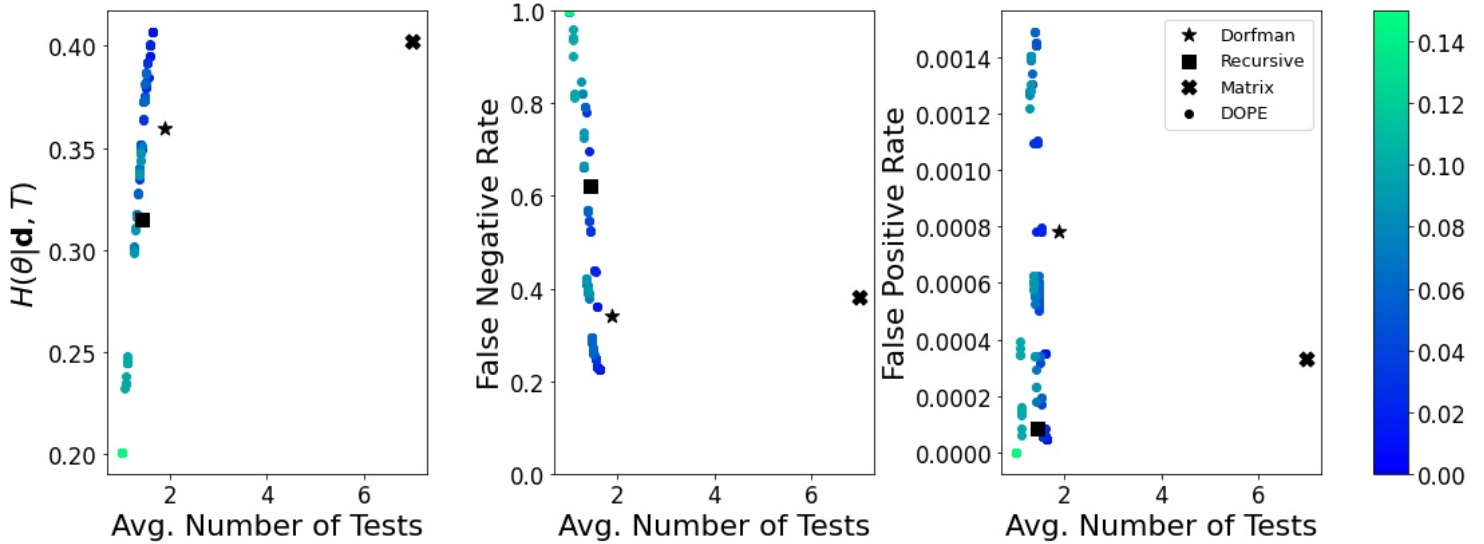

Figure 3: False-negative rates of DOPE, compared to two competing strategies with varying test parameters. Population is assumed iid. In the left panel shown are simulation results for  $P_{fp} = 0.01$  and in the right  $P_{fp} = 0.01$ . The test false-negative rate  $P_{fn}$  is plotted in both panels on the Y axis.

### 4 Reproducing results with false-positive rates

We present here figures from the main text. Figure 2 is reproduced with false-positive data in Figure 4.

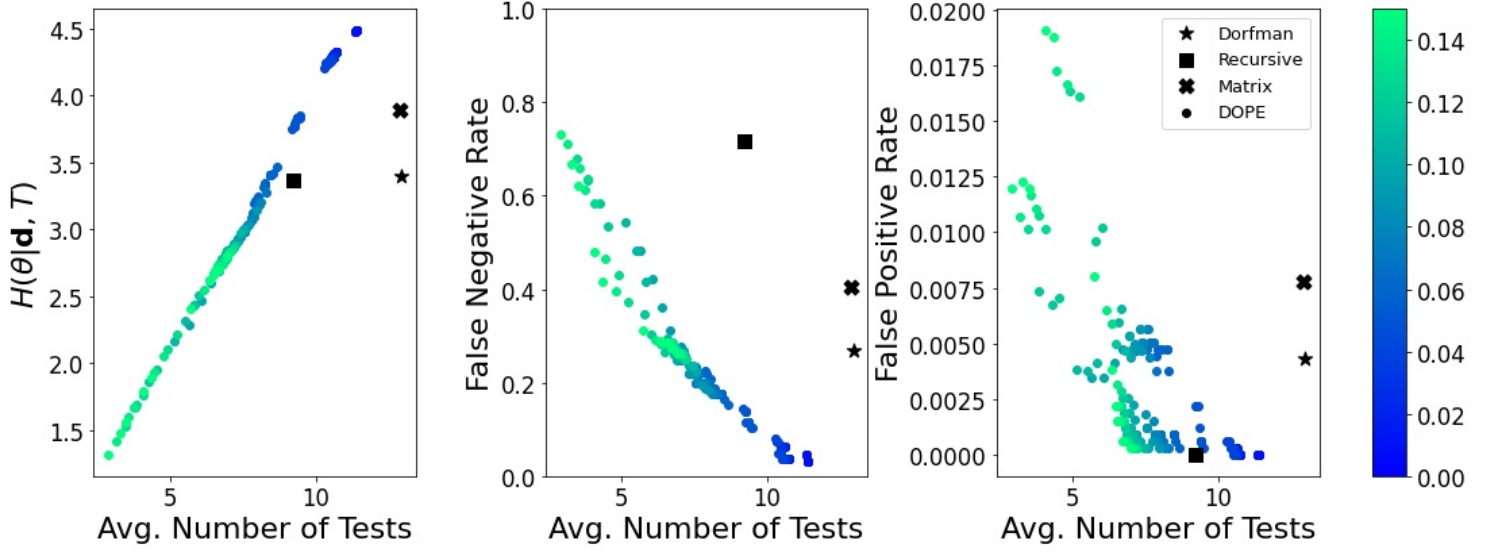

Figure 4: Results for population of size  $N = 32$ , reproduced with false-positive rates.

Figure 3 of the main text is reproduced with posterior entropy and false-positive data in Figure 5.

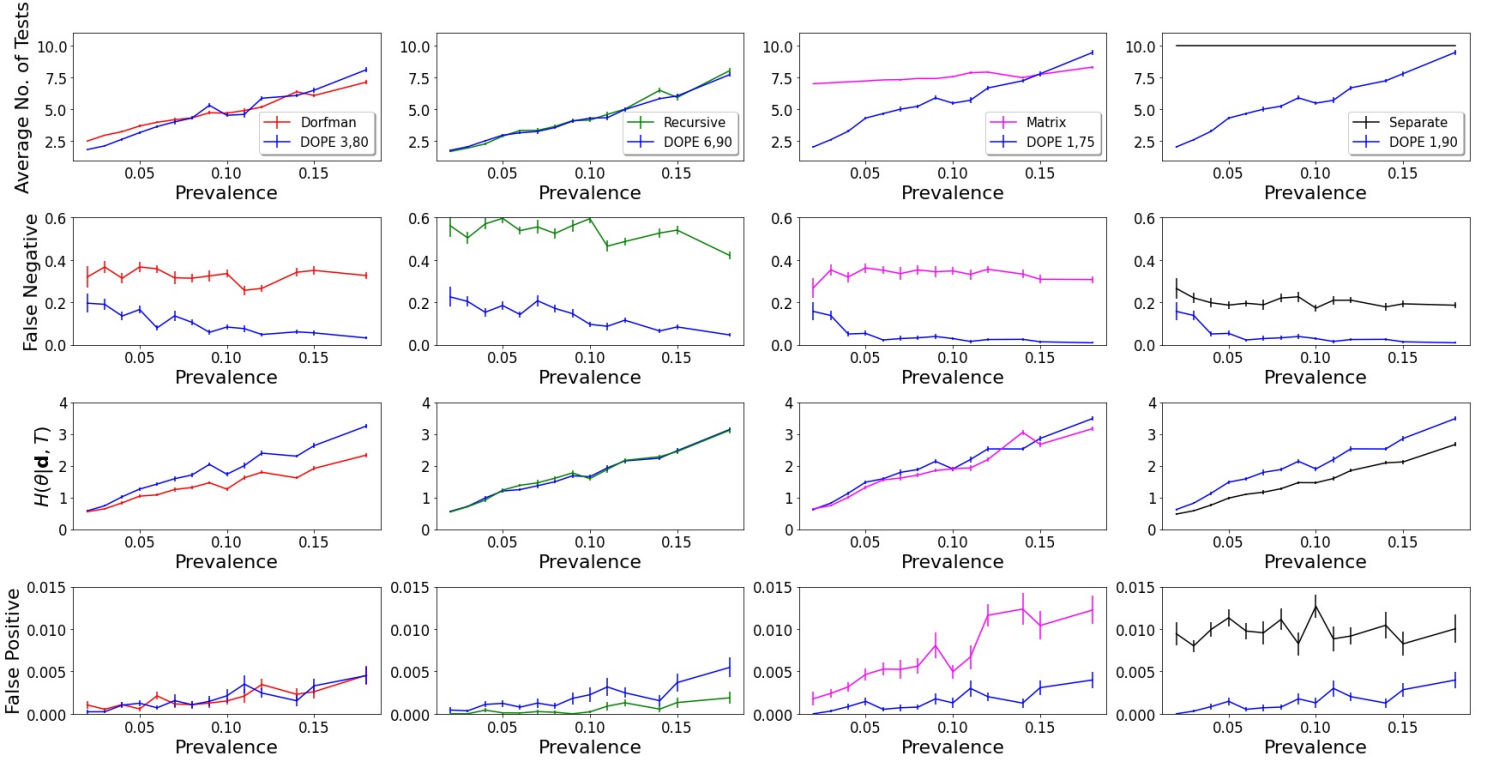

Figure 5: Comparison of DOPE for varying prevalence rates, reproduced to show false-positive rates.

## 5 Number of Monte Carlo simulations

We estimate the variance of  $\hat{\Psi}$  for a population of size  $N = 64$  with  $L = 20000$  simulations. We see it is fairly safe to take  $L = 20000$  simulations so we do this for populations of size  $N = 32$  also.

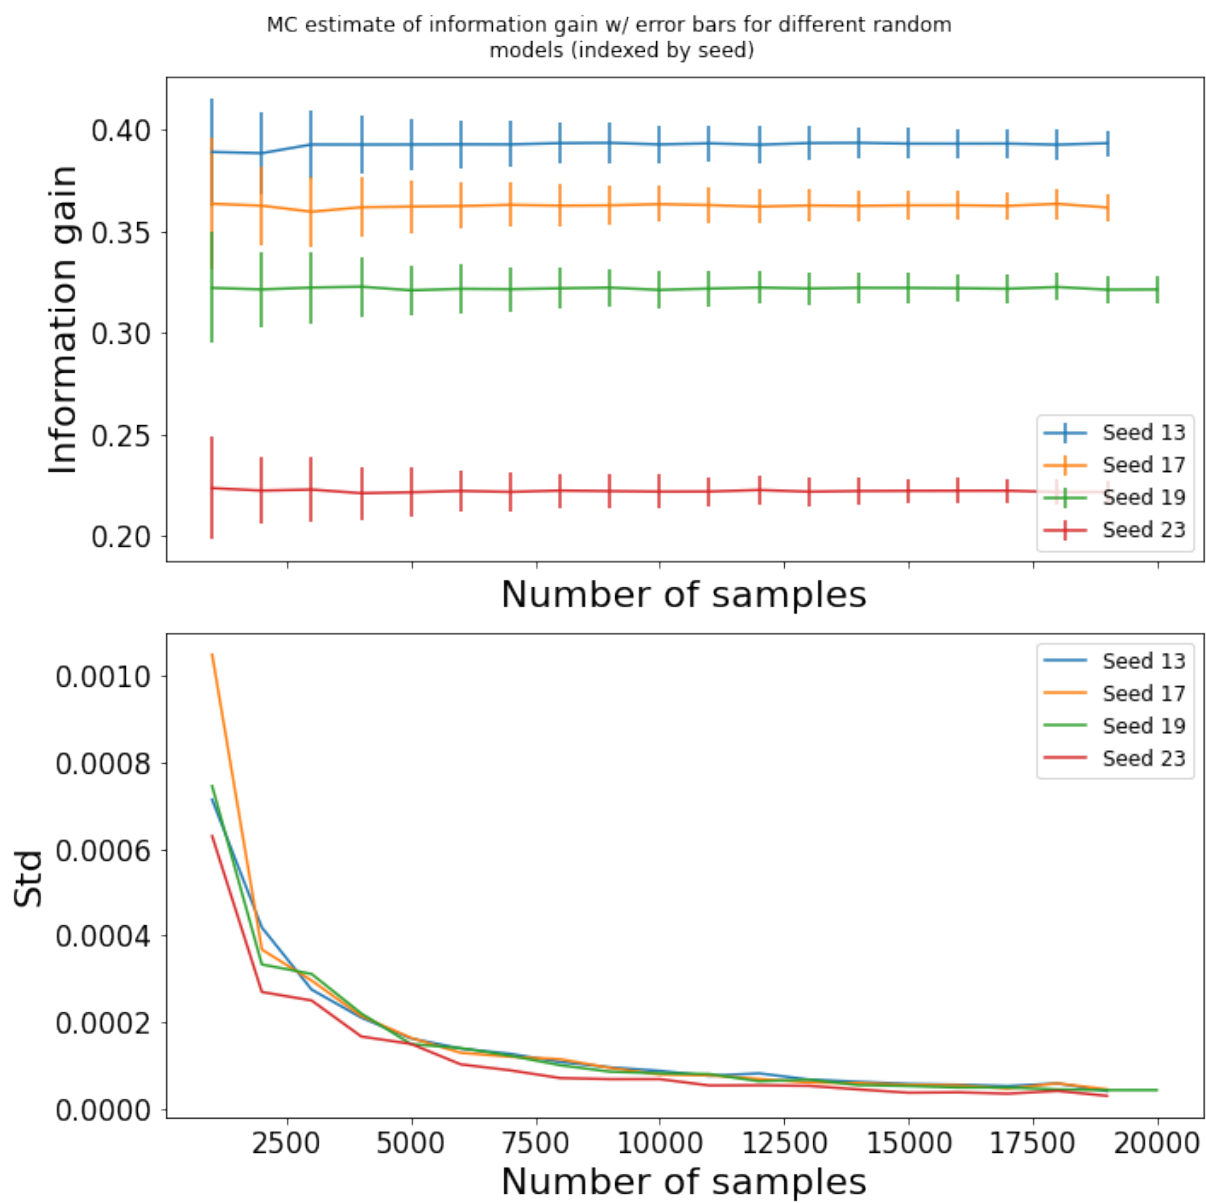

Figure 6: Monte Carlo estimates and standard deviation for estimation of mutual information for four random designs.

## 6 Implementing competing strategies

In **Dorfman** pooling, we partition the population to some number of pools and each pool is tested. If a pool test result is positive — each member of said pool is tested individually. An individual tested positive in the second test is declared positive. It is not clear what to do if all separate tests were negative for some pool. In our implementation, we did not take any special action, thus declaring all individuals in said pool negative. An optimal pool size that depends on disease prevalence in the tested population as suggested in [1] was taken.

**Recursive** pooling proceeds by pooling the maximal number of individuals allowed. The pool is tested and, upon a positive result — split in two. The process continues and an individual is declared positive if they are separately tested positive. If a pool test result is negative at any point — all pool members are declared negative. It is not clear what to do if the first pool test result is positive, yet upon subsequent splitting and testing, two negative results are returned. In this case our implementation of recursive pooling takes no special action, and all pool members are declared negative.

In **matrix** pooling, we order a population of size  $N = k\ell$  in a matrix of size  $k \times \ell$ . Pools are formed and tested for each row and each column. If two or more column pools and two or more row pools are tested positive — individuals in the intersections are tested separately. If only one row or column is positive — there is no need for subsequent testing. It is not clear what should be done if, e.g. all rows are negative yet some column is positive. Should we test each column member separately? Retest each row? Declare all individuals negative? Again, our approach takes no special action and in this case all population members are declared negative.

## 7 Considering secondary infection probabilities

We simulate two households of size 5. In the first we consider our connectivity model. In the second, we allow secondary infection of household members if at least one basal infection took place. The difference between prevalences were negligible — 0.7%. We conclude that our prior model, though simplistic, does capture the essence of population connectivity.

## 8 Parameter Estimates

In this section we collect some results regarding the reliability of pooling and population connectivity. These are used in the simulations we run and the results.

### 8.1 Pool sizes

In [9], the authors suggest using pools up to size 30 individuals is reasonable and has little effect on false-negative rates. The authors of [16] suggest using pool sizes as large as 64. According to [13], dilution has negligible effect on RT-PCR results. There, it was shown that a 1000 time dilution of samples still yields Ct below 35.

### 8.2 SARS-CoV-2 RT-PCR error rates

A pooling study [2] cites false positive rates close to 5%. This figure pertains to pools of size 5 and 8. Ct values increased as expected from theory ( $\log_2 n$ , for  $n$  the dilution factor).

According to [13], false-negative rates ranged from 23% (10 out of 13) to 8% (12 out of 13). Notably, the same authors also mention that cross reactivity with other coronaviruses is almost non-existent.

Another study [12] cites false-negative rates of 2%- 29% (citing 37% false-negative rate for nasal swabs). No reference was made to false-positive rates.

Another study [14] estimated the false-negative rate as a function of days from symptom onset. The estimate was 6% for day 0 and 33% on day 10. These figures are true for nasal swabs.

Yet another study [6] cites false-negative rates of 100% on the day following an infection to 67% on the fourth day (assumed last day before symptom onset). On the day of symptom onset, false-negative rate is estimated at 58% and three days after symptom onset this decreases to 20%.

A study [15] used 5% as false-positive rate. A different study [11] estimated false-positive rate at 1.2%.

An lower bound for test false-negative and false-positive is 5%, according to [10]. One study [3] estimated false-negative rate at 1% and false-positive rate at 0.2%.

### 8.3 Secondary infection estimates

A study in China [5] cites 17% probability of infection in the same residential address.

Another study [8] cites 515 infected of total 11,580 contacts. This amounts to 4.4% infection. Attack rates for close family members are cited as  $20.68 \cdot 4.4\% = 91\%$  for spouses and  $9.55 \cdot 4.4\% = 42\%$  for non spouse family members.

A study conducted in the US states of Tennessee and Wisconsin cites secondary infection rate of 53% [4].

A study conducted in China [7] cites secondary attack rates in household to be 16.3%. Other attack rates include 27% (spouse), 17% (adult household non-spouse members), and 4% (non-spouse children in household).

One study [3] estimated false-negative rate at 1% and false-positive rate at 0.2%.

## 9 Description of table in Supplementary Material B

The attached table gives a detailed account of connectivity parameters  $P_p, P_s, P_b$  we used to generate populations and their corresponding prevalences. Column names are self explanatory.

## References

- [1] Hrayr Aprahamian, Douglas R Bish, and Ebru K Bish, *Optimal group testing: Structural properties and robust solutions, with application to public health screening*, INFORMS Journal on Computing (2020).
- [2] Netta Barak, Roni Ben-Ami, Tal Sido, Amir Perri, Aviad Shtoyer, Mila Rivkin, Tamar Licht, Ayelet Peretz, Judith Magenheimer, Irit Fogel, et al., *Lessons from applied large-scale pooling of 133,816 SARS-CoV-2 RT-PCR tests*, Science Translational Medicine (2021).
- [3] Ana Paula Christoff, Giuliano Netto Flores Cruz, Aline Fernanda Rodrigues Sereia, Dellyana Rodrigues Boberg, Daniela Carolina de Bastiani, Lais Eiko Yamanaka, Gislaine Fongaro, Patricia Hermes Stoco, Maria Luiza Bazzo, Edmundo Carlos Grisard, et al., *Swab pooling for large-scale RT-qPCR screening of SARS-CoV-2*, Available at SSRN 3689590 (2020).
- [4] Carlos G Grijalva, *Transmission of SARS-CoV-2 infections in households—Tennessee and Wisconsin, April–September 2020*, MMWR. Morbidity and Mortality Weekly Report **69** (2020).

- [5] Qin-Long Jing, Ming-Jin Liu, Zhou-Bin Zhang, Li-Qun Fang, Jun Yuan, An-Ran Zhang, Natalie E Dean, Lei Luo, Meng-Meng Ma, Ira Longini, et al., *Household secondary attack rate of COVID-19 and associated determinants in Guangzhou, China: a retrospective cohort study*, The Lancet Infectious Diseases (2020).
- [6] Lauren M Kucirka, Stephen A Lauer, Oliver Laeyendecker, Denali Boon, and Justin Lessler, *Variation in false-negative rate of reverse transcriptase polymerase chain reaction—based SARS-CoV-2 tests by time since exposure*, Annals of Internal Medicine (2020).
- [7] Wei Li, Bo Zhang, Jianhua Lu, Shihua Liu, Zhiqiang Chang, Peng Cao, Xinhua Liu, Peng Zhang, Yan Ling, Kaixiong Tao, et al., *The characteristics of household transmission of COVID-19*, Clinical Infectious Diseases (2020).
- [8] Tao Liu, Wenjia Liang, Haojie Zhong, Jianfeng He, Zihui Chen, Guanhao He, Tie Song, Shaowei Chen, Ping Wang, Jialing Li, et al., *Risk factors associated with COVID-19 infection: a retrospective cohort study based on contacts tracing*, Emerging microbes & infections **9** (2020), no. 1, 1546–1553.
- [9] Stefan Lohse, Thorsten Pfuhl, Barbara Berkó-Göttel, Jürgen Rissland, Tobias Geißler, Barbara Gärtner, Sören L Becker, Sophie Schneitler, and Sigrun Smola, *Pooling of samples for testing for SARS-CoV-2 in asymptomatic people*, The Lancet Infectious Diseases (2020).
- [10] C Mayers and K Baker, *Impact of false-positives and false-negatives in the UK’s COVID-19 RT-PCR testing programme*, 2020.
- [11] Nikhil S Padhye, *Reconstructed diagnostic sensitivity and specificity of the RT-PCR test for COVID-19*, medRxiv (2020).
- [12] Jessica Watson, Penny F Whiting, and John E Brush, *Interpreting a COVID-19 test result*, BMJ **369** (2020).
- [13] L Wijsman, R Molenkamp, CBEM Reusken, A Meijer, et al., *Comparison of seven commercial RT-PCR diagnostic kits for COVID-19*, Journal of clinical virology: the official publication of the Pan American Society for Clinical Virology **128** (2020), 104412–104412.
- [14] Paul Wikramaratna, Robert S Paton, Mahan Ghafari, and Jose Lourenco, *Estimating false-negative detection rate of SARS-CoV-2 by RT-PCR*, medRxiv (2020).

- [15] Steven Woloshin, Neeraj Patel, and Aaron S Kesselheim, *False negative tests for SARS-CoV-2 infection-challenges and implications*, New England Journal of Medicine (2020).
- [16] Idan Yelin, Noga Aharony, Einat Shaer Tamar, Amir Argoetti, Esther Messer, Dina Berenbaum, Einat Shafran, Areen Kuzli, Nagham Gandali, Omer Shkedi, et al., *Evaluation of covid-19 rt-qpcr test in multi sample pools*, Clinical Infectious Diseases **71** (2020), no. 16, 2073–2078.
